# Supplementary material for: LitAR: Visually Coherent Lighting for Mobile Augmented Reality
Source: arXiv:2301.06184 source file (2023-01-15)
Supplement: Supplementary file 2 [file fig_render_1.tex]

\begin{figure}
  \includegraphics[width=0.95\linewidth]{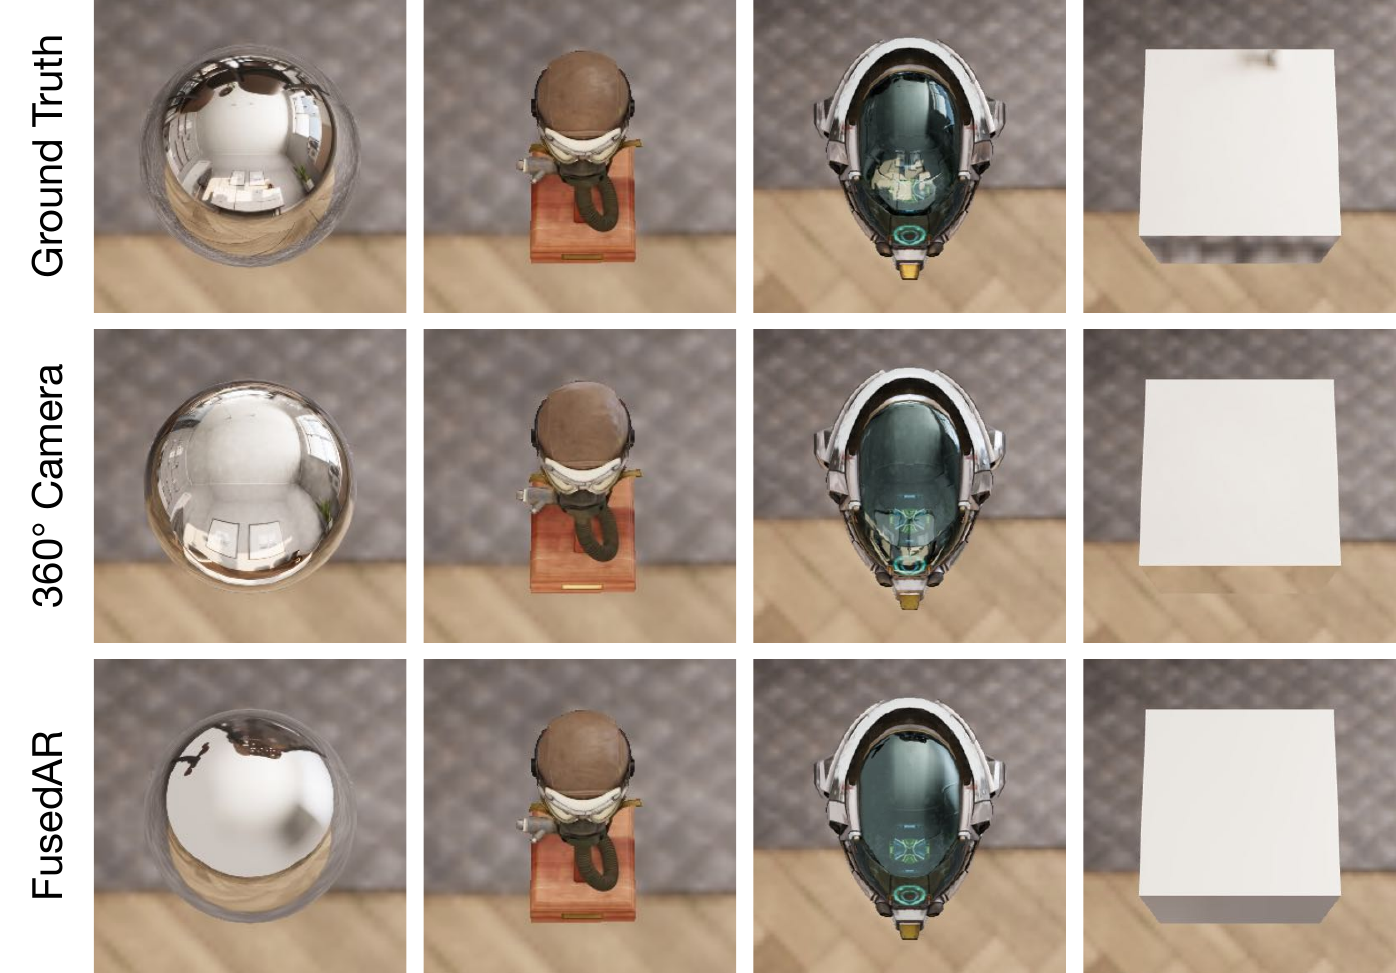}
%   \vspace{-0.5em}
  \caption{Full rendering comparison of row one in teaser image.
  }
%   \label{fig:full_col}
%   \vspace{-1.5em}
\end{figure}
